# Supplementary material for: DReAM: Dynamic Reconfigurable Architecture Modeling (full paper)
Source: arXiv:1805.03724 source file (2018-10-23)
Supplement: Supplementary file 1 [file appendix.tex]

\section*{Appendix}
	
	\subsection*{Abbreviations for Interaction Constraints}
	The following abbreviations extend and/or generalize what has been presented in \ref{sec:interaction-constraints}:
	\begin{itemize}
		\item \emph{causal constraint}: used to specify the ports required for the interaction involving the local port $p$.
		More specifically, we can require that a set of component instances $\left\lbrace B_1,\dots,B_n \right\rbrace $ satisfying constraint $\varPsi$ must jointly participate, respectively, with ports $q_1,\dots,q_n$ in the interaction via the abbreviation:
		\begin{align*}
			\mathbf{Require}& \ q_1^{j_1} \ \dots \ q_n^{j_n} \left[ B_1[j_1] \ \dots \ B_n[j_n]  \ | \ \varPsi(j_1,\dots,j_n) \right]  \equiv \\
			&\exists B_1[j_1] : \ \dots \ \exists B_n[j_n] : \varPsi(j_1,\dots,j_n) \wedge q_1^{j_1} \wedge \dots \wedge q_n^{j_n}
		\end{align*}
		\item \emph{acceptance constraint}: allows optional ports $q_1,\dots,q_n$ of component instances $\left\lbrace B_1,\dots,B_n \right\rbrace $, respectively, satisfying the FOIL formula $\varPsi$ to participate in the interaction involving the local port $p$ by explicitly excluding all the non-optional ports and all the ports that do not satisfy $\varPsi$:
		\begin{align*}
			\mathbf{Accept}& \ q_1^{j_1} \ \dots \ q_n^{j_n} \left[ B_1[j_1] \ \dots \ B_n[j_n] \ | \ \varPsi(j_1,\dots,j_n) \right] \equiv \\
			& \bigwedge_{(B_h,q) \notin \left\lbrace (B_1,q_1),\dots,(B_n,q_n) \right\rbrace} \forall B_h[j] : \left( q^j \neq p^{\mathtt{self}} \Rightarrow (q^j \Rightarrow \mathtt{false}) \right) \ \wedge \\
			& \forall B_1[j_1]: \dots \forall B_n[j_n] : \neg \varPsi(j_1,\dots,j_n) \Rightarrow \left( (q_1^{j_1} \vee \dots \vee q_n^{j_n}) \Rightarrow \mathtt{false} \right)
		\end{align*}
		\item \emph{filtering constraints}: require that ports $q_1,\dots,q_n$ of component instances $\left\lbrace B_1,\dots,B_n \right\rbrace $, respectively, satisfying the FOIL formula $\varPsi$ participate in the interaction with at most/least\footnote{although the notation may appear counter-intuitive, note that $\mathbf{AtLeast}(k) \ \phi \nRightarrow \mathbf{Require} \ \phi$, in that the only interactions that are filtered are the ones including ports in $\phi$; e.g. the constraint $\mathbf{AtLeast}(2) \ q^j [B[j] \ | \ \mathtt{tt}]$ is satisfied by interactions including at least two instances of port $q$ or not including any port $q$ at all} a set amount instances per port name $q_i$:
		\begin{align*}
			\mathbf{AtMost}(k)& \ q_1^{j_1} \ \dots \ q_n^{j_n} \left[ B_1[j_1] \ \dots \ B_n[j_n] \ | \ \varPsi(j_1,\dots,j_n) \right] \equiv \\
			&\forall B_1[j_1]: \forall B_1[j_{11}] : \dots \forall B_1[j_{1k}] : \dots \forall B_n[j_n] : \forall B_n[j_{n1}]: \dots \forall B_n[j_{nk}] : \\
			&\varPsi(j_1,\dots,j_n) \Rightarrow \bigwedge_{i=1}^{n} \left( \left(q^{j_i} \wedge \bigwedge_{h=1}^{k} q^{j_ih}\right) \Rightarrow \bigvee_{h=1}^{k} j_i = j_{ih} \right)
		\end{align*}
		\begin{align*}
			\mathbf{AtLeast}(k)&  \ q_1^{j_1} \ \dots \ q_n^{j_n} \left[ B_1[j_1] \ \dots \ B_n[j_n] \ | \ \varPsi(j_1,\dots,j_n) \right] \equiv \\
			&\dots
		\end{align*}
		Additionally we can express the generalised $\mathbf{Unique}$ constraint over $n$ ports and the $\mathbf{Exactly}(k)$ abbreviation as follows:
		\begin{align*}
		\mathbf{Unique}& \ q_1^{j_1} \ \dots \ q_n^{j_n} \left[ B_1[j_1] \ \dots \ B_n[j_n] | \varPsi(j_1,\dots,j_n) \right]  \equiv \\
		&\forall B_1[j_1]: \forall B_1[{j'}_1] : \dots \forall B_n[j_n] : \forall B_n[{j'}_n] : \\ 
		&\varPsi(j_1,\dots,j_n) \Rightarrow ((q_1^{j_1} \wedge q_1^{j'_1} \Rightarrow j_1 = j'_1) \wedge \dots \wedge (q_n^{j_n} \wedge q_n^{j'_n} \Rightarrow j_n = j'_n)) 
		\end{align*}
		\begin{align*}
		\mathbf{Exactly}(k)  \ q_1^{j_1} \ \dots \ q_n^{j_n} \left[ B_1[j_1] \ \dots \ B_n[j_n] \ | \ \varPsi(j_1,\dots,j_n) \right] \equiv
		\mathbf{AtMost}(k) \wedge \mathbf{AtLeast}(k)
		\end{align*}
	\end{itemize}
%	\newpage
%	\subsection*{Grammars}
%	
%	\subsubsection*{Attributes, instance ids and port fields}
%	Let $n \in \mathbb{N}$, $p \in \mathcal{P}$ and $\ell \in \mathfrak{L}$.
%	$$ \mathsf{Attr} ::= \mathsf{Iid} \ | \ \mathsf{Pf} \ | \ n $$
%	$$ \mathsf{Iid} ::= n $$
%	$$ \mathsf{Pf} ::= p.\ell$$
%	
%	\subsubsection*{Port expressions}
%	Let $n \in \mathbb{N}$, $p \in P \subset \mathcal{P}$ and $\ell \in \mathfrak{L}$.
%	$$ \mathsf{Pexp}_P ::= p.\ell \ | \ n \ | \ \mathsf{Pexp}_P \ \mathsf{op} \ \mathsf{Pexp}_P $$
%	where $\mathsf{op} ::= + \ | \ - \ | \ * \ | \ \div$.
